# Supplementary material for: Diversely Regularized Matrix Factorization for Accurate and Aggregately Diversified Recommendation
Source: arXiv:2211.01328 source file (2022-10-19)
Supplement: Supplementary file 1 [file 090appendix.tex]

\onecolumn
\section{Additional Experiments}
\label{sec:AdditionalExp}
%\nopagebreak

\begin{figure*}[h]
	\centering
	\subfigure{\includegraphics[width=0.45\textwidth]{./FIG/performance/perf_legend}}\\\vspace{-3mm}

	\subfigure{\includegraphics[width=0.95\textwidth]{./FIG/performance/perf_top10}}
	
	\caption{
		Accuracy-diversity trade-off curves of top-$10$ recommendations in each dataset.
		\method draws the best curves which are closer to the best point compared to those of other competitors.
	}
	\label{FIG:appendix_perf10}
\end{figure*}

% \begin{figure*}[h]
% 	\centering
% 	\subfigure{\includegraphics[width=0.45\textwidth]{./FIG/performance/perf_legend}}\\\vspace{-3mm}
	
% 	\subfigure{\includegraphics[width=0.95\textwidth]{./FIG/performance/perf_top20}}
	
% 	\caption{
% 			Accuracy-diversity trade-off curves of top-$20$ recommendations in each dataset.
% 		\blue{
% 			UImatch shows the highest coverage in Yelp-15, Gowalla-15, and ML-10M since it forces rarely recommended items to be recommended with strict capacity constraints.
% 			However, \method achieves higher entropy than UImatch because the capacity constraints of UImatch are skewed to maintain the recommendation accuracy so that the recommendation lists of UImatch are also skewed.
% 			In summary, \method shows the best overall performance compared to other competitors.
% 		}
% 	}
% 	\label{FIG:appendix_perf20}
% \end{figure*} 
